# Supplementary material for: RobustPeriod: Time-Frequency Mining for Robust Multiple Periodicity Detection
Source: arXiv:2002.09535 source file (2021-03-08)
Supplement: Supplementary file 1 [file 7_Appendix.tex]

% \section{Appendix: proof of Proposition \ref{prop:HuberPeriodogram_dist}}
\section{Proof of Proposition 3}
We first refer readers to the \textit{General Theorem} and \textit{Theorem 1} in \cite{li2010nonlinear}, based on which we are able to prove that with the additional assumption $e)$ in Proposition~\ref{prop:HuberPeriodogram_dist}, the results in both theorems still hold for our Huber loss function.

\textit{General Theorem \cite{li2010nonlinear}:} Let ${\mu_t}$ and ${c_{jt}}$ be bounded deterministic sequences. Let $\{X_t\}$ satisfy the assumptions (a) and (b) in Theorem 1. Assume further that there exist positive-definite matrices $\mathbf{Q_0}$ and $\mathbf{W_0}$ such that $\mathbf{Q_n} := diag\{\mathbf{Q_{jn}}\}_{j=1}^{q} \ge \mathbf{Q_0}$ and $\mathbf{W_n} := [\mathbf{W_{jkn}]_{j,k=1}^q} \ge \mathbf{W_0}$ for large $n$. Then, as $n \rightarrow \infty$, $\sqrt{n}\text{vec}\{\hat{\beta}_{jn}-\beta_{j0}-\mathbf{\theta}_{jn}\}_{j=1}^q \stackrel{A}{\sim} N(0,\mathbf{\Gamma_n})$, where $\mathbf{\theta}_{jn} := \mathbf{Q}_{jn}^{-1}\mathbf{b}_{jn}$ and $\mathbf{\Gamma}_n := \mathbf{Q}_n^{-1}\mathbf{W}_n\mathbf{Q}_n^{-1}$, where
\begin{align}
    \mathbf{b}_{jn} :=& n^{-1} \sum_{t=1}^n E\{g_p(U_{jt})\}c_{jt},\\
    \mathbf{W}_{jkn} :=& n^{-1} \sum_{t=1}^n\sum_{s=1}^n Cov\{g_p(U_{jt}), g_p(U_{ks})\}c_{jt}c_{ks}^T,\\
    \mathbf{Q}_{jn} :=& n^{-1}\sum_{t=1}^nE\{h_p(U_{jt})\}c_{jt}c_{jt}^T,\\
    g_p(x) :=& |x|^{p-1}sgn(x),\\
    h_p(x) :=& (p-1)|x|^{p-2}.
\end{align}{}
With an additional assumption that $n_1 \ge n_2^2$, where $n_1, n_2$ represent the length of the sequence that $|Y_t - c_t^T\beta| \le \theta$ and $|Y_t - c_t^T\beta| > \theta$, respectively. Note that $n_1 + n_2 = n$. We are able to show that this \textit{General Theorem} still hold for the Huber loss case. 
\begin{proof}
The key step is to reformulate the optimization problem for $\mathbf{\beta}$ to $\mathbf{\delta}$, and split the objective function as two parts, i.e., one in $L_2$ and one in $L_1$ form. With additional assumption $n_1 \ge n_2^2$, we can show that $L_1$ part in the objective function is asymptotically close to $o_P(1)$, where $o_P(1)$ represents a term that approaches zero in probability. As a result, the remaining $L_2$ part can be approximated by a quadratic function and an asymptotically Gaussian term using the similar argument as in \cite{li2010nonlinear}. 

To get the optimal regression coefficient $\hat{\beta}_n$, we need to solve optimization problem $\hat{\beta}_n = \text{argmin}_\beta \sum |Y_t - \mathbf{c}_t^T\beta|$, and the total error becomes $U_t:= Y_t - \mathbf{c}_t^T\beta_0 = X_t - e_t$, where $e_t := \mathbf{c}_t^T\beta_0 - \mu_t$. Because $Y_t = U_t +  \mathbf{c}_t^T\beta_0$, it follow that $\hat{\beta}_n$ also minimizes $\frac{1}{2}\sum^{n_1} {|U_t - v_t(\delta)|^2 - |U_t|^2} + \frac{1}{2}\sum^{n_2} {|U_t - v_t(\delta)| - |U_t|}$, with $\delta := \sqrt{n}(\beta-\beta_0)$, this problem can be reformulated as
\begin{multline} % \begin{multline} equation
    Z_n(\delta) = \frac{1}{2}\sum^n_{t=1} \left(|U_t - v_t(\delta)|^2 - |U_t|^2\right) + \\ \frac{1}{2}\sum^n_{t=2} \left(|U_t - v_t(\delta)| - |U_t|\right),
\end{multline}{\label{eq:reformualte-opt}}
where $v_t(\delta):=c_t^T\delta/\sqrt{n}$. 
We now want to show that 
\begin{equation}
    Z_n(\delta) = \Tilde{Z}_n(\delta) + o_P(1)
\end{equation}{}
for fixed $\delta \in R^r$. Based on Lemma 2.8 in \cite{arcones2001asymptotic}, since the (vii) result in Lemma 2.8 holds for both $p=1$ and 2, we are able to show that
\begin{multline}
    \Tilde{Z}_n(\delta) = \frac{1}{2}\sum^{n_1} \{-g_2(u)v + \frac{1}{2}h_2(u)v^2 + r_1(u,v)\} + \\
    \sum^{n_2} \{-g_1(u)v + \frac{1}{2}h_1(u)v^2 + r_2(u,v))\},
\end{multline}{}
where
$r_i(u,v) := \text{min}\{|u|^{p-3}|v|^3,|u|^{p-2}|v|^2\}$. Similar to \cite{li2010nonlinear}, we can rewrite the above equation for $\Tilde{Z}_n(\delta)$ as $T_{1n}+T_{2n}+T_{3n}$, where $T_{1n}:= -\sum_{n_1} g_2(u)v$, $T_{2n}:= -\frac{1}{2} \sum_{n_1} h_2(u)v^2$, and $T_{3n} := \sum^{n_1} r_1(u,v) + \sum^{n_2} \{-g_1(u)v + r_2(u,v))\}$. Next, we focus on to show that $T_{3n}$ is asymptotically negligible. The proof of $T_{2n}$ can be approximated by a quadratic function and $T_{1n}$ is asymptotically Gaussian can be derived using the same argument in \cite{li2010nonlinear} for $p=2$.\\
To prove $\frac{1}{2}\sum^{n_1} r_1(u,v)+ \sum^{n_2} r_2(u,v)$ asymptotically goes to $o_P(1)$, we borrow the upper bounds that have been derived for $r_i(u,v), i=1,2$ by \cite{li2010nonlinear}, i.e.,
\begin{align}
    E\{r_0(U_t,v_t)\} \le &v_t^2 \cdot ( f_0 \int_{|x| \le |v_t|} |x|^{p-2} dx \\
    &+ f_0 v_t \int_{|x| \ge |v_t|} |x|^{p-3} dx).
\end{align}{}
The above bounds do not exist for general case when $p=1$ or 2, but given our piece-wise nature of Huber loss, we are able to show that for both $p = 1$ and $p=2$, the terms in parenthesis above is finite. Therefore, $E\{r_0(U_t,v_t)\}$ is bounded by $o_P(n^{-1})$. \\
Given the assumption that $n_1 \ge n_2^2$, then $\sum^{n_2} -g_1(u)v$ is $o_P(1)$. We omit the rest of the proof and refer readers to \cite{li2010nonlinear}.

\end{proof}
