# Supplementary material for: RobustPeriod: Time-Frequency Mining for Robust Multiple Periodicity Detection
Source: arXiv:2002.09535 source file (2021-03-08)
Supplement: Supplementary file 2 [file 8_Supple_rPeriod.tex]

\section{Appendix}
% \section{ADMM for Huber-Periodogram and Complexity Analysis}
\subsection{Implementation Overview}
In this section, we describe the implementation of the proposed robustPeriod algorithm. 

Our robustPeriod algorithm is implemented with Python, where 
the H-P filter is based on statsmodels\footnote{Seabold, Skipper, and Josef Perktold. “statsmodels: Econometric and statistical modeling with python.” Proceedings of the 9th Python in Science Conference. 2010.},
the MODWT is based on the PyWavelets\footnote{Gregory R. Lee, Ralf Gommers, Filip Wasilewski, Kai Wohlfahrt, Aaron O’Leary (2019). PyWavelets: A Python package for wavelet analysis. Journal of Open Source Software, 4(36), 1237, https://doi.org/10.21105/joss.01237.}, 
the DFT/IDFT based on Scipy\footnote{Virtanen, P., Gommers, R., Oliphant, T.E. et al. SciPy 1.0: fundamental algorithms for scientific computing in Python. Nat Methods (2020). https://doi.org/10.1038/s41592-019-0686-2.}, and 
the peak detection of ACF is based on signal.find\_peaks in Scipy.

For the parameters of different components in robustPeriod algorithm, we adopt a fixed configurations for all experiments in the paper. It works quit well as shown in experiment section in the paper, which also makes our robustPeriod widely deployed in different  applications in Alibaba. 
Specifically, the time series is normalized by mean and variance in H-P filter and its $\lambda$ is set as $10^{-6}$ in Eq.~\eqref{eq:hp_trend}. The MODWT is set as Daubechies-4. In the Huber-Periodogram, the result of $\boldsymbol{\phi} \boldsymbol{\beta} -  \mathbf{x}$ in Eq.~\eqref{eq:Periodogram_final} is normalized by mean and variance before the operation of Huber function where the threshold in Huber is set as $\zeta=1$ in Eq.~\eqref{eq:huber_loss}, and the threshold in Fisher test in Section~\ref{sec:RobustFisher} is set as $\alpha=10^{-10}$. In the peak detection of normalized ACF in Section~\ref{sec:RobustACF}, we set the threshold as 0.5. The normalization in H-P filter and Huber function makes the parameter setting simple and can be used in a wide of time series. 

Note that for most parts of the proposed robustPeriod algorithm, their implementation is straightforward based on the formulation in the paper, except the solution of the proposed Huber-Periodogram which is described in details in the following subsection.

\subsection{Implementation of Huber-Periodogram}
\subsubsection{ADMM formulation}
We apply ADMM to solve the proposed Huber-Periodogram. Firstly we reformulate the optimization problem of Huber-Periodogram in Eq.~\eqref{eq:Periodogram_final} as
\begin{eqnarray}\label{eq:Periodogram_admm}
& \min &   \gamma_{\zeta}^{hub} ( \mathbf{z})\\
& ~~~\text{s.t.}\quad & \boldsymbol{\phi} \boldsymbol{\beta} -  \mathbf{x}  = \mathbf{z}
\end{eqnarray}
Then we can obtain the augmented Lagrangian as
\begin{equation}\label{eq:Lagrangian} \notag
L_{\rho}(\boldsymbol{\beta},\mathbf{z},\mathbf{v}) = 
\gamma_{\zeta}^{hub}(\mathbf{z}) +
\mathbf{v}^T ( \boldsymbol{\phi} \boldsymbol{\beta} -  \mathbf{x}  - \mathbf{z}) + \frac{\rho}{2} || \boldsymbol{\phi} \boldsymbol{\beta} -  \mathbf{x}  - \mathbf{z}||_2^2
\end{equation}
where $\mathbf{v}$ is the dual variable, and $\rho$ is the penalty parameter.
Following the ADMM procedure~\cite{boyd2011distributed} and taking proximal operator for huber function $\gamma_{\zeta}^{hub} ( \mathbf{z})$~\cite{Parikh2014}, we can obtain the updating steps as
\begin{align} % \label{eq:admm}
\boldsymbol{\beta}^{k+1} ={}&  (\boldsymbol{\phi}^T \boldsymbol{\phi} )^{-1} \boldsymbol{\phi}^T (\mathbf{z}^k+\mathbf{x}-\mathbf{u}^k)\label{eq:admm1}\\
\begin{split} 
\mathbf{z}^{k+1} ={}& \frac{\rho}{1+\rho}\left( \boldsymbol{\phi} \boldsymbol{\beta}^{k+1} + \mathbf{u}^{k}  - \mathbf{x} \right) +  \\
 & \frac{1}{1+\rho}S_{\frac{\zeta(1+\rho)}{\rho}}\left( \boldsymbol{\phi} \boldsymbol{\beta}^{k+1} + \mathbf{u}^{k}  - \mathbf{x}  \right) 
\end{split}\label{eq:admm2}\\
\mathbf{u}^{k+1} ={}& \mathbf{u}^{k} +  \boldsymbol{\phi} \boldsymbol{\beta}^{k+1} - \mathbf{z}^{k+1}- \mathbf{x}  \label{eq:admm3}
\end{align}
where $\mathbf{u}=(1/\rho)\mathbf{v}$ is the scaled dual variable to make the formulation more convenient.
The soft thresholding operation ${S}_{\rho}(x)$ in $\mathbf{z}-$minimization step can be efficiently calculated by %${S}_{\rho}(x) = (1-\rho/|x|)_{+}x$.
\begin{equation}\label{eq:soft_thresholding} 
{S}_{\rho}(x) =
\begin{cases} 
0,       & |x| \leq \rho\\
x- \rho \text{sgn}(x), & |x| > \rho
\end{cases}
\end{equation}

For the termination criteria, besides the maximum iteration number, we also check the primal and dual residuals in each ADMM iteration until they are small enough. Specifically, the values of primal residual $\mathbf{r}^k$ and dual residual $\mathbf{s}^k$ at $k$th iteration are calculated by
\begin{align}\label{eq:primal:residual}
\|\mathbf{r}^k\|_2 &= \|\boldsymbol{\phi} \boldsymbol{\beta}^{k} - \mathbf{z}^k\ - \mathbf{x}\|_2,\\
\|\mathbf{s}^k\|_2 &= \rho \|\boldsymbol{\phi}^T (\mathbf{z}^k - \mathbf{z}^{k-1})\|_2.
\end{align}
Then, $\|\mathbf{r}^k\|_2$ and $\|\mathbf{s}^k\|_2$ are checked if they are smaller than the corresponding tolerance thresholds as~\cite{boyd2011distributed}
\begin{align}   
\epsilon^{pri} &= \sqrt{N} \epsilon^{abs} + \epsilon^{rel}\max\{\|\boldsymbol{\phi} \boldsymbol{\beta}^{k}\|_2, \|\mathbf{z}^{(k)}\|_2,  \|\mathbf{x}\|_2 \},\label{eq:tol_pri} \\
\epsilon^{dual} &= \sqrt{2}\epsilon^{abs} + \epsilon^{rel}\|\rho \boldsymbol{\phi}^T \mathbf{u}^{(k)}\|_2,\label{eq:tol_dual}
\end{align}
where $\epsilon^{abs}>0$ is an absolute tolerance and $\epsilon^{rel}>0$ is a relative tolerance. 

\subsubsection{Parameter Setting}
The threshold of Huber function in~\eqref{eq:Periodogram_admm} is set as $\zeta=1$. And the threshold of soft thresholding in~\eqref{eq:admm2} is set as $\rho=1$. Both absolute tolerance $\epsilon^{abs}$and relative tolerance $\epsilon^{rel}$ are set as $10^{-4}$ in~\eqref{eq:tol_pri}, \eqref{eq:tol_dual}. Besides the termination criteria, we also set the maximum number of ADMM iteration in~\eqref{eq:admm1} to \eqref{eq:admm3} as 50. 

% where 
% The  is set as  
% % 
% % \eqref{eq:Periodogram_admm}
% % \rho} \label{eq:soft_thresholding} 
% % \label{eq:admm1}  2 3 
% % 50  

% %  {eq:tol_pri}  \label{eq:tol_dual}   \epsilon^{abs}   \epsilon^{rel}
% % A reasonable choice for the two tolerance in our case is around $10^{-3}$ to $10^{-4}$.
% % rel_par=1.,
%                         % tol_abs=1e-5,
%                         % tol_rel=1e-2):

\subsubsection{Complexity Analysis}
For the complexity of the ADMM in Huber-Periodogram, we can obtain $\mathcal{O}(N)$ computational complexity for each iteration based on Eq.~\eqref{eq:admm1} to Eq.~\eqref{eq:admm3} (note that $\boldsymbol{\phi}$ is an $N \times 2$ matrix). Furthermore, we can store the value of $(\boldsymbol{\phi}^T \boldsymbol{\phi} )^{-1} \boldsymbol{\phi}^T$ in Eq.~\eqref{eq:admm1} to save time since it is unchanged in each iteration. For required number of iteration, we can get $\epsilon$-optimal solution within $\mathcal{O}(N/\epsilon)$ iterations~\cite{boyd2011distributed}. Note that in our case, the ADMM often converges well within a few tens of iterations.

% the number of iterations required is $\mathcal{O}(N/\epsilon)$, where $\epsilon$ is the error between the solver and optimal solution. 
% For the computational complexity of each iteration (updating step) in ADMM, we can obtain $\mathcal{O}(N)$ complexity based on the updating steps in Eq.~\eqref{eq:admm1} to Eq.~\eqref{eq:admm3} (note that $\boldsymbol{\phi}$ is an $N \times 2$ matrix). 

% $\epsilon$-optimal solution within $\mathcal{O}(N/\epsilon)$ iterations

% \section{Temp}
% % \addtocounter{proposition}{2} % this is for appendix with right numbering
% sdf

% \bibliographystyle{aaai}
% %\bibliography{yourbibfile1,yourbibfile2}
% \bibliography{6_Periodicity_bibfile}

% \end{document}
